# Supplementary material for: Towards Quantifying the Distance between Opinions
Source: arXiv:2001.09879 source file (2020-01-27)
Supplement: Supplementary file 1 [file supplementary.tex]

\documentclass[11pt,a4paper]{article}
\usepackage[hyperref]{emnlp-ijcnlp-2019}

\usepackage{times}
\usepackage{latexsym}

\usepackage{url}
\usepackage{booktabs} % For formal tables
\usepackage{algorithm}
\usepackage{algpseudocode}%
\usepackage{multirow}
\usepackage{tabularx}
\usepackage{comment}
\usepackage{graphicx}
\usepackage{amsmath}
\usepackage{tabularx}
\newcolumntype{L}{>{\raggedright\arraybackslash}X}

\title{Supplementary: Towards Quantifying the Distance between Opinions}

\begin{document}
\maketitle

%\vspace{-1em}

In this supplementary material, we discuss the finer details of our proposed opinion distance framework and empirical setup along with additional experimental results and observations.

\section{Methods}
\label{baselines}
In this section, we explain the selected baselines and the parameter setting for benchmarking the performance of the competing approaches. \\

\noindent \textbf{1. TF-IDF:} The distance between two opinions is computed as the cosine distance between their term-frequency inverse-document frequency (TF-IDF) vectors of those opinions~\cite{schutze2008introduction}. Following standard practice, we remove the stop words while computing the TF-IDF. We note that in spite of its simplicity, TF-IDF is an incredibly effective baseline for such tasks. \\

\noindent \textbf{2. WMD:} The distance between two text documents can be captured using the recently proposed Word Mover Distance (WMD)~\cite{kusner2015word} -- which in our setting would enable the capture of the distance between opinions. %Following the methodology laid out by the original authors, 
We use a pre-trained word2vec embedding~\cite{mikolov2013efficient} trained on GoogleNews Corpus for computing the WMD. Note that WMD, in this baseline, is used to compute the text-similarity between all words in the two opinion texts (except stopwords) and is, thus, used as a text-similarity measure. 

In contrast, our usage of WMD within the opinion distance computation framework is to match the noun phrases or disambiguated concepts present within the opinion representations in order to collate and compare the associated sentiment polarities. Observe, that since WMD is a specialized case of Earth Mover Distance which requires the whole mass of one sentence to be morphed into the mass of another sentence, setting uniform weight values for opinion subjects was seen to mitigate this problem in our setting. \\

\noindent \textbf{3. Sent2vec:} The distance between two opinions %in this baseline relies on the computation of 
is the cosine distance between Sent2vec~\cite{pgj2017unsup} embeddings of those opinions. We lever the pre-train sent2vec-wiki-unigrams model %available at Sent2vec github repo \footnote{https://github.com/epfml/sent2vec}
for computing sentence embeddings. \\

\noindent \textbf{4. Doc2vec:} The distance between two opinions %in this baseline relies on the computation of 
is the cosine distance between Doc2vec~\cite{le2014distributed} embeddings of those opinions. We pre-train the Doc2vec methodoogy on Wikipedia articles.

\section{System specifications} All the experiments in our empirical settings were conducted on a
machine running Linux with an Intel Xeon E5-2680 CPU (28 cores, 2.40GHz) and 128 GB of RAM.

\section{Opinion Distance Drilldown}
\label{exp:all_topics}
\input{table_case_study.tex}
In this section, we present a detailed drilldown of our proposed opinion distance measure.
We consider the following two variants of our measure:
{\em OD-d2v} and {\em OD-w2v} where the semantic distance is computed as cosine distance over Doc2vec embeddings (pre-trained on Wikipedia) and Word2vec embeddings (pre-trained on Google) respectively. The semantic threshold for OD-d2v is set at $0.3$ while for OD-w2v is set at $0.6$. In both the variants, we use the sentiment polarity shifters, a complete list of which are presented in Table~\ref{polarity_shifters}. 

%In addition to the above, we consider the following baselines that we have previously described; WMD (which relies on word2vec embeddings), Doc2vec and TF-IDF. 
We evaluate our distance measures in the unsupervised setting, specifically, evaluating the clustering quality using Adjusted Rand Index (ARI) and Silhouette coefficient. 
We benchmark against the following baselines: WMD (which relies on word2vec embeddings), Doc2vec and TF-IDF. The results are shown in Table~\ref{table:all_topics}, where we observe the following trends:

\textbf{1.} Opinion distance methods generally outperform the competition on both ARI and Silhouette coefficient. We observe that given a topic, the opinion distance measure is able to separate pro stance opinions from the con stance opinions. We also find that the other baselines generally perform worse as both pro and con stance opinions have high text similarity in many of these datasets. This is reflected in the average ARI and average Silhouette coefficients of the baseline distance measures.

\textbf{2.} On a few datasets, there are a few discriminating words between the different opinion clusters. For instance, in the topic ``Trade Union", the opinion subject ``collective bargaining" is contained in 60 \% of claims in the con stance of the topic while it is not present in the pro stance opinions on the topic. The pro stance opinions on this topic use the term ``Unions" as the opinion subject. Another example is ``Hydroelectric Dams" dataset, where 36 \% of pro stance opinions contain term "hydro" while only 18\% of con stance opinions contain term ``hydro". On such datasets, TF-IDF and WMD perform relatively better in separating pro stance opinions from the con stance opinions. In the exceptional case of ``Hydroelectric Dams" dataset, the opinion distance $OD$ performs particularly bad compared to TF-IDF because of some errors with disambiguation.

\begin{table}
\resizebox{0.95\linewidth}{!}{
\begin{tabular}{p{\linewidth}}
\toprule
\textbf{List of sentiment polarity shifters} \\ \toprule
\small{
'no', 'not', 'negation', 'none', "n't", 'inconclusive', 'without', 'excluded', "incompatible", "prevent", 'exacerbate',   'reduce',  'less', 'rarely',  'displaced', 'relocation', 'dislocation', 'higher than', 'relocate', 'resettled', 're-housed', 'cannot', 'limit', 'outweigh', 'unless', 'little act', 'get even'} \\ 
\toprule
\end{tabular}
}

\caption{Sentiment polarity shifters used across all datasets. \looseness=-1}

\label{polarity_shifters}

\end{table}

\input{table_polarity.tex}

\section{Variants of opinion distance}

%In this section, 
We compare the different variants of opinion distance. The polarity of opinion subject $pol(S_{i})$ can be represented in the form of absolute value or polarity distribution.  The results are shown in Table~\ref{tab:variants}. We make the following observations.

\noindent \textbf{1. $OD$ significantly outperforms $OD$-$parse$:} In line with the experiments reported later, we observe that $OD$ is not only computationally faster compared to $OD$-$parse$, it is also much more accurate. On the three datasets %of "Seanad abolition", "Video Games" and "Pornography"
, $OD$ achieves an average weighted F1 score of 0.53, 0.51 and 0.41 respectively compared to the scores of 0.01, -0.01 and 0.07 by $OD$-$parse$. This is largely because of the errors in dependency parsing and the resultant poor opinion representation.

\noindent \textbf{2. Representing polarities in form of distribution is inefficient:} We find that irrespective of the chosen variant of opinion distance, if we represent $pol(S_{i})$ in the form of distribution, we do not find good opinion clusters. The $D$ value of opinion distance calculated using polarity distribution is also low. Recall that Jensen-Shannon divergence is the distance measure used ~\citep{FSSY12}. Table~\ref{tab:variants} shows that $OD$ is significantly better than Jensen-Shannon divergence on all the three datasets.
%Note that this representation of polarities in form of distribution is tied to sentiment lexicon being used.

%This observation is orthogonal to the observation COM ~\citep{FSSY12} topic model where topics are first discovers 
\noindent \textbf{3. Sentiment polarity shifters have high impact on clustering performance of opinion distance: } We find that not utilizing the sentiment polarity shifters, specially in case of datasets ``Video games" and ``Pornography" hurts the {\it Opinion Representation} phase, and thereby leads to incorrect computation of opinion distance. This is evident from the significant drop in ARI score from $OD$ to $OD$ (no polarity shifters) since the only change in those variants is of sentiment polarity shifters.

\section{Unsupervised setting: Cluster Distance}

\label{sec:unsupervised_cluster_distance}
%In previous section, we measured the efficacy of distance measure based on cluster quality found using clustering methods. 
The measurement of efficacy of distance measure using clustering methods depends on the clustering method. Since the ground truth clusters are available, one way of measuring the efficacy of distance measure is to compare the intra-cluster  and inter-cluster distances. A good distance measure should have small intra-cluster distance and large inter-cluster distance. Let $I_k$ denote the intra-cluster distance for opinion cluster $C_k$ and $I'_k$ denote the inter-cluster distance for $C_k$, then $I_k$ and $I'_k$ are defined as follows:

\begin{align}
I_k & =  \sum_{i \in C_k}\sum_{\substack{j \in C_k \\ i \neq j}} distance \; (i,j)  \\
I'_k & =  \sum_{i \in C_k}\sum_{\substack{j \in C_l \\ k \neq l}} distance \; (i,j) 
\end{align}
\begin{comment}
\begin{equation}
I_k =  \sum_{i \in C_k}\sum_{j \in C_k; i \neq j} distance \; (i,j)
\end{equation}
%\frac{1}{{|C_k| \choose 2}}
\begin{equation}
I'_k =  \sum_{i \in C_k}\sum_{j \in C_l; k \neq l} distance \; (i,j)
\end{equation}
\end{comment}
We summarize intra-clusters/inter-clusters information in two measures, specifically micro and macro measures. However, in order to save space, we only report micro values but the trend of macro values is similar to that of micro values.  The absolute values of $I_k$ and $I'_k$ would have different interpretation for different distance measures, therefore we report the percent difference between inter-cluster and intra-cluster with respect to intra-cluster. We refer to the percent difference value for both micro/macro measures  as $D$ and report this value. Another way to address the disparity among distance measure values is to compute Silhouette coefficient \cite{rousseeuw1987silhouettes} based on ground truth cluster labels.  %The higher the value of $D$, the better the distance measure for opinions. 
The comparison of distance measures based on $D$ metric and Silhouette coefficient is shown in Table~\ref{table:cluster_quality_macro}. 

%The silhouette coefficient of a single opinion $i$ is computed using mean intra-cluster distance $a(i)$ and mean nearest-inter-cluster distance $b(i)$. Silhouette coefficient of opinion $i$ is $b(i)-a(i)/max(a(i),b(i))$. The final silhouette coefficient is mean of silhouette coefficient of all opinions\cite{scikit-learn}. Silhouette coefficient lies between -1 to 1 and higher values of silhouette coefficient refers to better opinion distance measure. The comparison of distance measures based on silhouette coefficient is shown in Table~\ref{table:cluster_quality_macro}. 
We make the following observations.

\begin{table}[t]
\input{table_clusters.tex}

\caption{We measure the quality of identified opinion cluster using Adjusted Rand Index (ARI).}
\label{table:cluster_result}
%\vspace{-2em}
\end{table}

\begin{table}[t]
\resizebox{0.95\linewidth}{!}{
\def\arraystretch{1.0}%  1 is the default, change whatever you need
\begin{tabular}{@{}lrrrcrrrcrrr@{}}
\toprule
 & \multicolumn{2}{c}{\begin{tabular}[c]{@{}c@{}}Seanad \\ Abolition \end{tabular}} & & \multicolumn{2}{c}{\begin{tabular}[c]{@{}c@{}}Video \\ Games \end{tabular}} & & \multicolumn{2}{c}{Pornography}\\
\cmidrule{2-3} 
\cmidrule{5-6} 
\cmidrule{8-9} 
Methods & $D$ (mi)  & $Sil$  && $D$ (mi) & $Sil$  &&  $D$ (mi) & $Sil$ \\ 
 
%& (mi) &   && (mi) &  && (mi) &  \\
\midrule

TF-IDF  & 2.7 & 0.02 && 0.2 & 0.01 && 0.2 & 0.01 \\
WMD  & -1.3 & 0.01 && 0.5 & 0.01 && 0.6 & 0.01  \\
Sent2vec & 0.7 & -0.01 &&  1.8 & 0.06 && 2.5 & 0.02  \\
Doc2vec  & -0.9 & -0.03 && 0.3 & 0.01 && -0.7 & -0.01  \\
OD-parse & -1.2 & -0.04 &&  -2.3 & 0.02 && 10.0  & 0.05  \\
OD & \textbf{147.5} & \textbf{0.31}  && \textbf{70.5} & \textbf{0.42} && \textbf{120.9} & \textbf{0.41} \\

\bottomrule
\end{tabular}
}
\caption{We measure the quality of distance measure by quantifying the percent difference between intra-cluster and inter-cluster distance along with Silhouette coefficient. }
\label{table:cluster_quality_macro}
%\vspace{-3em}
\end{table}

\noindent \textbf{1. {\it \textbf{OD}} correctly captures similarity and dissimilarity between opinions:} From Table~\ref{table:cluster_quality_macro}% and \ref{table:silhouette}
, we see that the opinion distance $OD$ has significantly large values of percent difference between inter and intra cluster distance values as well as significantly large values of Silhouette coefficient across three datasets. We see a similar trend in our detailed analysis in Table~\ref{table:all_topics}.

\noindent \textbf{2. Existing measures cannot differentiate similar opinions from dissimilar opinions:} From Table~\ref{table:cluster_result}, we found that for the ``Seanad Abolition" dataset, the performance of TF-IDF using clustering methods is relatively better than the other baselines. However, from Table~\ref{table:cluster_quality_macro}% and \ref{table:silhouette}
, we see that for TF-IDF both the macro and micro values of metric $D$ as well as the silhouette coefficient of TF-IDF are significantly lower than that of $OD$. This indicates that even though the TF-IDF distance measure itself had little value in discriminating between the different opinion clusters, the clustering methods k-means and spectral partitioning, 
could still leverage it to achieve the  relatively better clustering performance.
%\vspace{-1em}

\section{Supervised setting: Experimental Setup}
 For all the classification experiments, unless otherwise noted, we use SVM as classifier with RBF kernel.
We perform hyperparameter tuning using both grid search (with 5-fold cross validation)  and auto-sklearn~\cite{NIPS2015_5872} (with default `holdout' strategy). We use two tuning strategies because we face the problem of overfitting for smaller datasets using only one of the tuning strategy. Since we use two tuning strategies, the hyperparameter tuning is done on train split (70\%) and we report the best results on test split (30\%) averaged over 3 runs. For evaluation, we rely on the average weighted F1 measure for classification accuracy.

%\vspace{-1em}
\section{Running Time}

In this section, we compare the running time of the distance measures. The results are shown in Table \ref{tabletime}. While reporting the running time of opinion distance, we report the overall computation time and the number in parenthesis represents the time required to compute the representation of an opinion. In case of $OD$, we assume that the responses from TagME REST API are already requested and stored. While reporting the Doc2vec computation time, we include the time required to infer the embedding of each opinion once. We observe that by avoiding the computationally intensive part of dependency parsing, $OD$ is significantly faster than $OD$-$parse$. %Furthermore, 
We can also see that the time required to compute the opinion distance $OD$ is comparable to that of computing distances using Doc2vec.
\begin{table}[t]

\centering
\resizebox{0.90\linewidth}{!}{

\begin{tabular}{@{}lrrrr@{}}
\toprule
{Baselines} & \begin{tabular}[c]{@{}c@{}}  Seanad \\ Abolition \end{tabular} &  
 \begin{tabular}[c]{@{}c@{}} Video \\ Games \end{tabular} & 
 Pornography  \\

\toprule

{TF-IDF} & 0.01 & 0.02 & 0.01 \\
{WMD} & 1.3 & 9.3 & 1.4 \\
{Sent2vec} & 0.01 & 0.01 & 0.01 \\
{Doc2vec} & 20 & 45 & 15 \\
{OD-parse} & 213 (199) & 367 (322) & 192 (183)\\
{OD} & 19 (2.2) & 31 (2.2) & 13 (2.2) \\
\toprule

\end{tabular}
}

\caption{We report the overall running time (in secs) of computing all-pair distance matrix for the baselines.} %The number in parenthesis represents the time required to generate opinion representation.}
\label{tabletime}
%\vspace{-3.4em}
\end{table}

\begin{comment}
\begin{tabular}{@{}lrrrr@{}}
\toprule
{Baselines} & \begin{tabular}[c]{@{}c@{}}  Seanad \\ Abolition \end{tabular} &  
 \begin{tabular}[c]{@{}c@{}} Video \\ Games \end{tabular} & 
Gambling & 
Pornography \\

\toprule

{TF-IDF} & 0.01 & 0.02 & 0.01 & 0.01 \\
{WMD} & 1.3 & 9.3 & 5.5 & 1.4 \\
{Doc2vec} & 20.5 & 45.5 & 31.4 & 15.7 \\
{OD-parse} & 213.6 (199.3) & 367.1 (322.4) & 279 (247) & 192 (183.7)\\
{OD} & 19.7 (2.2) & 31.4 (2.2) & 21.5 (2.2) & 12.9 (2.2) \\
\toprule

\end{tabular}
}
\end{comment}

\vspace{-0.5em}
\section{Case study}
%\vspace{-0.5em}
\input{case_study.tex}

\section{Noun-phrase Representation: SemRegex Rules }

The parse-tree variant of opinion distance $OD-parse$ relies lever dependency parse tree to extract opinion subject and opinion expression terms. In addition to the basic dependencies, enhanced dependencies and Named entity extraction functionalities present in Stanford CoreNLP, we also lever SemRegex rules. The list of rules with Stanford CoreNLP’s SemRegrex pattern matching system are presented in Table \ref{tab:semregex}. The $OpSubject$ refers to opinion subject while $OpExp#$ refers to the opinion expression. %Note that these rules can possibly result in few ``false positives"  %, however, the accuracy of rule-based system is typically better \cite{chiticariu2013rule}. 
%. Since the number of rules are limited, ``true positives" examples can possibly be missed. 

\begin{table*}[t]
    \centering
   \resizebox{0.95\linewidth}{!}{
   \small{
    \begin{tabular}{c|l}
    \toprule
         & \textbf{SemRegex Rules} \\
         \midrule
1 & $ \{\}=OpExp1 >/nmod:in/ \{\}=OpSubject$ \\
2 & $ \{\}=OpExp1 >/nmod:to/ \{\}=OpSubject$ \\
3 & $ \{\}=OpExp1 </nmod:of/ \{\}=OpSubject$ \\
4 & $ \{\}=OpExp1 >/nmod:by/ \{\}=OpSubject$ \\
5 & $ \{\}=OpExp1 >/nmod:after/ \{\}=OpSubject$ \\
6 & $ \{\}=OpExp1 >/nmod:without/ \{\}=OpSubject$ \\
7 & $ \{\}=OpExp1 >nsubj \{\}=OpSubject >dobj \{\}=OpExp2$ \\
8 & $ \{\}=OpExp1 >nsubj \{\}=OpSubject <csubj \{\}=OpExp2$ \\
9 & $ \{\}=OpExp1 >nsubj \{\}=OpSubject >/compound.*/ \{\}=OpExp2$ \\
10 & $ \{\}=OpExp1 </advcl:as/ \{\}=OpSubject$ \\
11 & $ \{tag:/VB.*/\} >nsubj \{\}=OpSubject  [ >acomp \{\}=OpExp1 | >xcomp \{\}=OpExp2]$ \\
12 & $ \{tag:/VB.*/\}=OpExp2 >advmod \{\}=OpExp1 [< \{\}=OpSubject | > \{\}=OpSubject]$ \\
13 & $ \{tag:/NN.*/\}  >nsubj \{\}=OpSubject  >amod \{\}=OpExp1$ \\
14 & $ \{tag:/NN.*/\}  >nsubj \{\}=OpSubject  >/nmod.*/ (\{\}=OpExp1 >amod \{\}=OpExp2$ \\
         \bottomrule
    \end{tabular}
    }
  }
    \caption{SemRegex Rules}
    \label{tab:semregex}
\end{table*}{}

\bibliographystyle{acl_natbib}
\bibliography{sample-bibliography}

\end{document}
